# Supplementary material for: PrivaScissors: Enhance the Privacy of Collaborative Inference through the Lens of Mutual Information
Source: arXiv:2306.07973 source file (2023-05-17)
Supplement: Supplementary file 1 [file appendix_threat.tex]

\section{Privacy Leakage in Collaborative Inference}\label{app:motivation}
\subsection{Data Leakage from the Representation}\label{sec:motivation_data}

\begin{wrapfigure}{r}{0.25\textwidth}
\centering
    \vspace{-5mm}
     \includegraphics[scale=0.3]{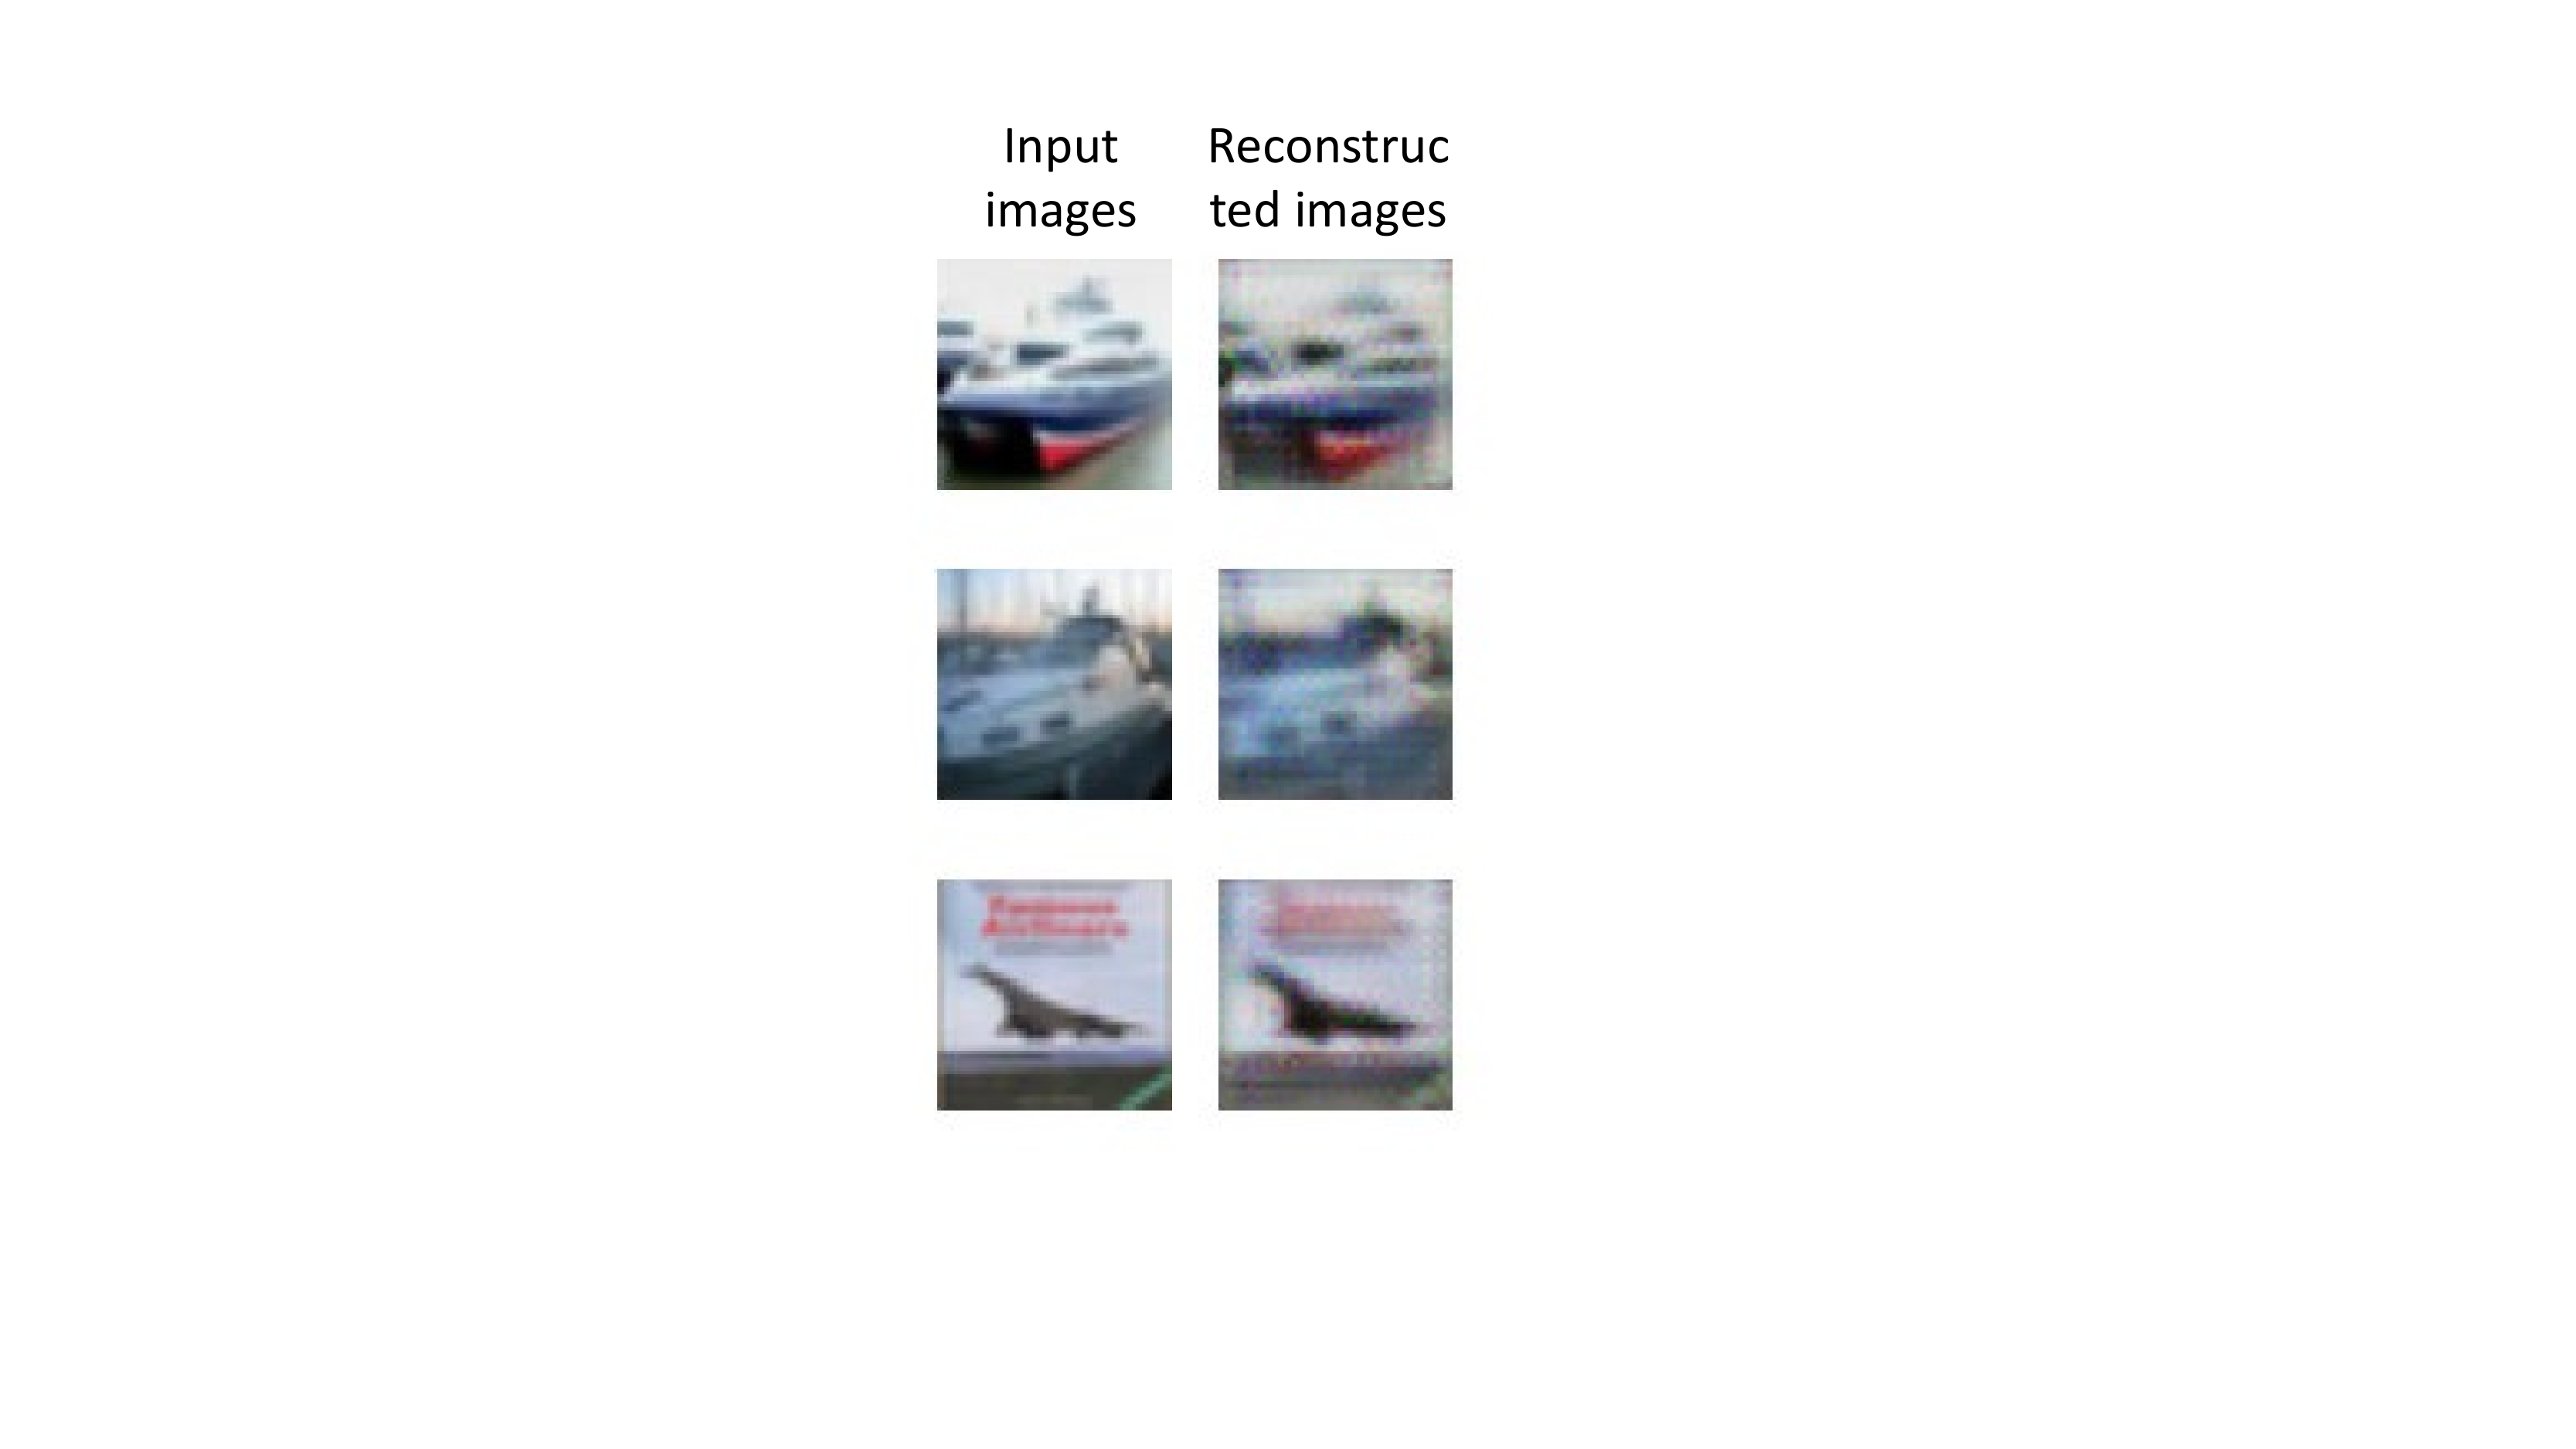}
\caption{Reconstructed images of KA attack.}
\vspace{-5mm}
\label{fig:motivation_KA}
\end{wrapfigure}

With the received representation $r_i$, the server can reconstruct the input data $x_i$ on the edge device by conducting model inversion (MI) attacks~\cite{}. Notably, the head model on the edge device is usually shallow due to the computation resource limitation, which aggravates data leakage vulnerability from the representation~\cite{}. We conduct experiments on CIFAR10 with ResNet18 to demonstrate the data leakage problem. One convolutional layer is deployed on the device as the head model, and one basic block is deployed as the classifier. The malicious server conducts Knowledge Alignment (KA) attack~\cite{} to recover the input image from the received representation through a generator. The detailed experimental settings can be found in Appendix~\ref{}. The reconstructed images are shown in \cref{fig:motivation_KA}. The high-quality reconstructed images illustrate the collaborative inference's vulnerability to the device's data leakage from the representation.

\subsection{Prediction Leakage from the Feature}

The training process enables the cloud server to extract high-level features useful for the collaborative inference task. These high-level features allow the malicious server to fine-tune a classifier head with very few labeled data and accurately conduct inference. The leakage of the prediction makes the edge device holder's privacy, including behavior and preference, exposed to the cloud server. For example, prediction leakage of a collaborative inference-based navigation mobile app allows the cloud server to infer the positions and destinations of the app users. To demonstrate the extent of prediction leakage by the features, we follow the experimental setup in \cref{sec:motivation_data} and let the cloud server conduct model completion (MC) attack~\cite{} to train a classifier using a small number of auxiliary labeled samples. We also let the cloud server train an entire model with the auxiliary dataset from scratch for comparison. The results are shown in \cref{tb:prediction_leakage}.

\begin{table}[th]
\small
    \centering
    \caption{Compared accuracy of the classifier on the device and the models on the cloud server by conducting MC attack and training from scratch.}
        \begin{tabular}{l | c }
            \toprule
            & Accuracy(\%)\\
            \hline
            Classifier on the device (clean accuracy) & 78.20\\
            \hline
            MC attack on the server(400 labels) & 74.90\\
            \hline
            Train from scratch on the server(400 labels) & \\
            \bottomrule
        \end{tabular}
    \label{tb:prediction_leakage}
\end{table}

It is shown that by fine-tuning a classifier with the collaboratively trained encoder, the cloud server can achieve comparable accuracy using an auxiliary dataset with only 400 labeled samples. However, training from scratch cannot achieve decent accuracy using the same auxiliary dataset, which shows that the high-level features extracted by the encoder on the server cause prediction leakage.
