# Supplementary material for: PrivaScissors: Enhance the Privacy of Collaborative Inference through the Lens of Mutual Information
Source: arXiv:2306.07973 source file (2023-05-17)
Supplement: Supplementary file 2 [file appendix_exp.tex]

\section{Additional Experimental Results}\label{app:experiments}
